# Supplementary material for: Beyond Theorems: A Counterexample to Potential Markov Game Criteria
Source: arXiv:2405.08206 source file (2024-05-13)
Supplement: Supplementary file 1 [file 8-appendix.tex]

\section{Proof of \reflmm{lemm:lemma1}}
\label{sec:proof-lemma-1}

\begin{proof}
 We prove the result by showing that for any state $s \in S$, the sequence:
 \[
  H^{t, \bm{\pi}}(s), H^{t+1, \bm{\pi}}(s), \dots
 \]
 is a Cauchy sequence.
 In other words, we show that for any state $s \in S$ and for any $\epsilon > 0$, there exists $T^\prime > 0$ such that for all $t^\prime, t^{\prime\prime} > T^{\prime}$, and any $\bm{\pi} \in \bm{\Pi}$, we have:
 \[
  \left\vert H^{t^\prime, \bm{\pi}}(s) - H^{t^{\prime\prime}, \bm{\pi}}(s) \right\vert < \epsilon.
 \]
 To this end, define $h^{\max} \triangleq \max_{s, \bm{a}} \vert h(s, a) \vert$.
 Suppose $t^\prime \geq t^{\prime\prime}$.
 Then for any state $s \in S$, we have:
 \begin{align*}
  \ifthenelse{\boolean{arxiv}}{
   H^{t^\prime, \bm{\pi}}(s) - H^{t^{\prime\prime}, \bm{\pi}}(s) &= \EE_{\bm{\pi}} \left[ \sum_{t=0}^{t^\prime - 1} \gamma^t h(s_t, \bm{a_t}) - \sum_{t=0}^{t^{\prime \prime} - 1} \gamma^t h(s_t, \bm{a_t}) \given[\Big] s_0 = s \right] \\
   &= \EE_{\bm{\pi}} \left[ \sum_{t=t^{\prime \prime}}^{t^\prime - 1} \gamma^t h(s_t, \bm{a_t}) \given[\Big] s_0 = s \right].
  }{
   H^{t^\prime, \bm{\pi}}(s) &- H^{t^{\prime\prime}, \bm{\pi}}(s) \\
   &= \EE_{\bm{\pi}} \left[ \sum_{t=0}^{t^\prime - 1} \gamma^t h(s_t, \bm{a_t}) - \sum_{t=0}^{t^{\prime \prime} - 1} \gamma^t h(s_t, \bm{a_t}) \given[\Big] s_0 = s \right] \\
   &= \EE_{\bm{\pi}} \left[ \sum_{t=t^{\prime \prime}}^{t^\prime - 1} \gamma^t h(s_t, \bm{a_t}) \given[\Big] s_0 = s \right].
  }
 \end{align*}
 By Cauchy-Schwartz inequality, we have: 
 \begin{align*}
  \left\vert H^{t^\prime, \bm{\pi}}(s) - H^{t^{\prime\prime}, \bm{\pi}}(s) \right\vert & = \left\vert \EE_{\bm{\pi}} \left[ \sum_{t=t^{\prime\prime}}^{t^\prime-1} \gamma^t h(s_t, \bm{a_t}) \given[\Big] s_0 = s \right] \right\vert \\
  & \leq \sum_{t=t^{\prime\prime}}^{t^\prime-1} \gamma^t h^{\max} \\
  & = \gamma^{t^{\prime\prime}} (1 - \gamma^{t^{\prime} - t^{\prime\prime}}) \left( \frac{h^{\max}}{1 - \gamma} \right) \\
  & \leq \gamma^{t^{\prime\prime}} \left( \frac{h^{\max}}{1 - \gamma} \right) \\
  & \leq \gamma^{T^\prime} \left( \frac{h^{\max}}{1 - \gamma} \right) \\
  & = e^{- T^{\prime} \vert \ln{\gamma} \vert } \left( \frac{h^{\max}}{1 - \gamma}\right).
 \end{align*}
 Therefore, to prove the result, we choose $T^\prime$ as follows:
 \[
  T^\prime > \left\vert \frac{\ln{(\epsilon \frac{1-\gamma}{h^{\max}})}}{\ln{\gamma}} \right\vert.
 \]
\end{proof}
